# Supplementary material for: Introducing the NewsPaLM MBR and QE Dataset: LLM-Generated High-Quality Parallel Data Outperforms Traditional Web-Crawled Data
Source: arXiv:2408.06537 source file (2024-11-23)
Supplement: Supplementary file 1 [file mbr_greedy_comparison.tex]

\begin{table*}[t]
    \centering
    \begin{adjustbox}{width=\textwidth}
\begin{tabular}{llcccc}
\toprule
& \bf Model & \bf BLEURT $\uparrow$ & \bf MetricX $\downarrow$ & \bf COMET20 $\uparrow$ & \bf COMET22 $\uparrow$ \\
\midrule
\multirow{2}{*}{\textit{en$\rightarrow$de}}
& MBR + QE finetuning (from greedy-pretrained ckpt) & \bf 70.48 & \bf 2.11 & \bf 55.39 & \bf 82.78 \\
& Greedy finetuning (from MBR + QE-pretrained ckpt) & 67.82 & 2.63 & 50.28 & 81.48 \\
\midrule
\multirow{2}{*}{\textit{de$\rightarrow$en}}
& MBR + QE finetuning (from greedy-pretrained ckpt) & \bf 72.44 & \bf 3.10 & \bf 58.58 & \bf 84.05 \\
& Greedy finetuning (from MBR + QE-pretrained ckpt) & 70.73 & 3.60 & 54.72 & 83.08 \\
\bottomrule
\end{tabular}
\end{adjustbox}
\caption{Comparison of pretraining on greedy data, then finetuning on MBR/QE data, vs vice-versa.}
\label{tab:mbr-greedy-all-metrics}
\end{table*}
